# Supplementary material for: Improving Convergence for Quantum Variational Classifiers using Weight Re-Mapping
Source: arXiv:2212.14807 source file (2023-02-15)
Supplement: Supplementary file 1 [file 8_appendix.tex]

\section*{\uppercase{Appendix}}

If any, the appendix should appear directly after the
references without numbering, and not on a new page. To do so please use the following command:
\textit{$\backslash$section*\{APPENDIX\}}

\begin{figure*}
     \centering
     \begin{subfigure}[t]{0.32\textwidth}
         \centering
         \includegraphics[width=\textwidth]{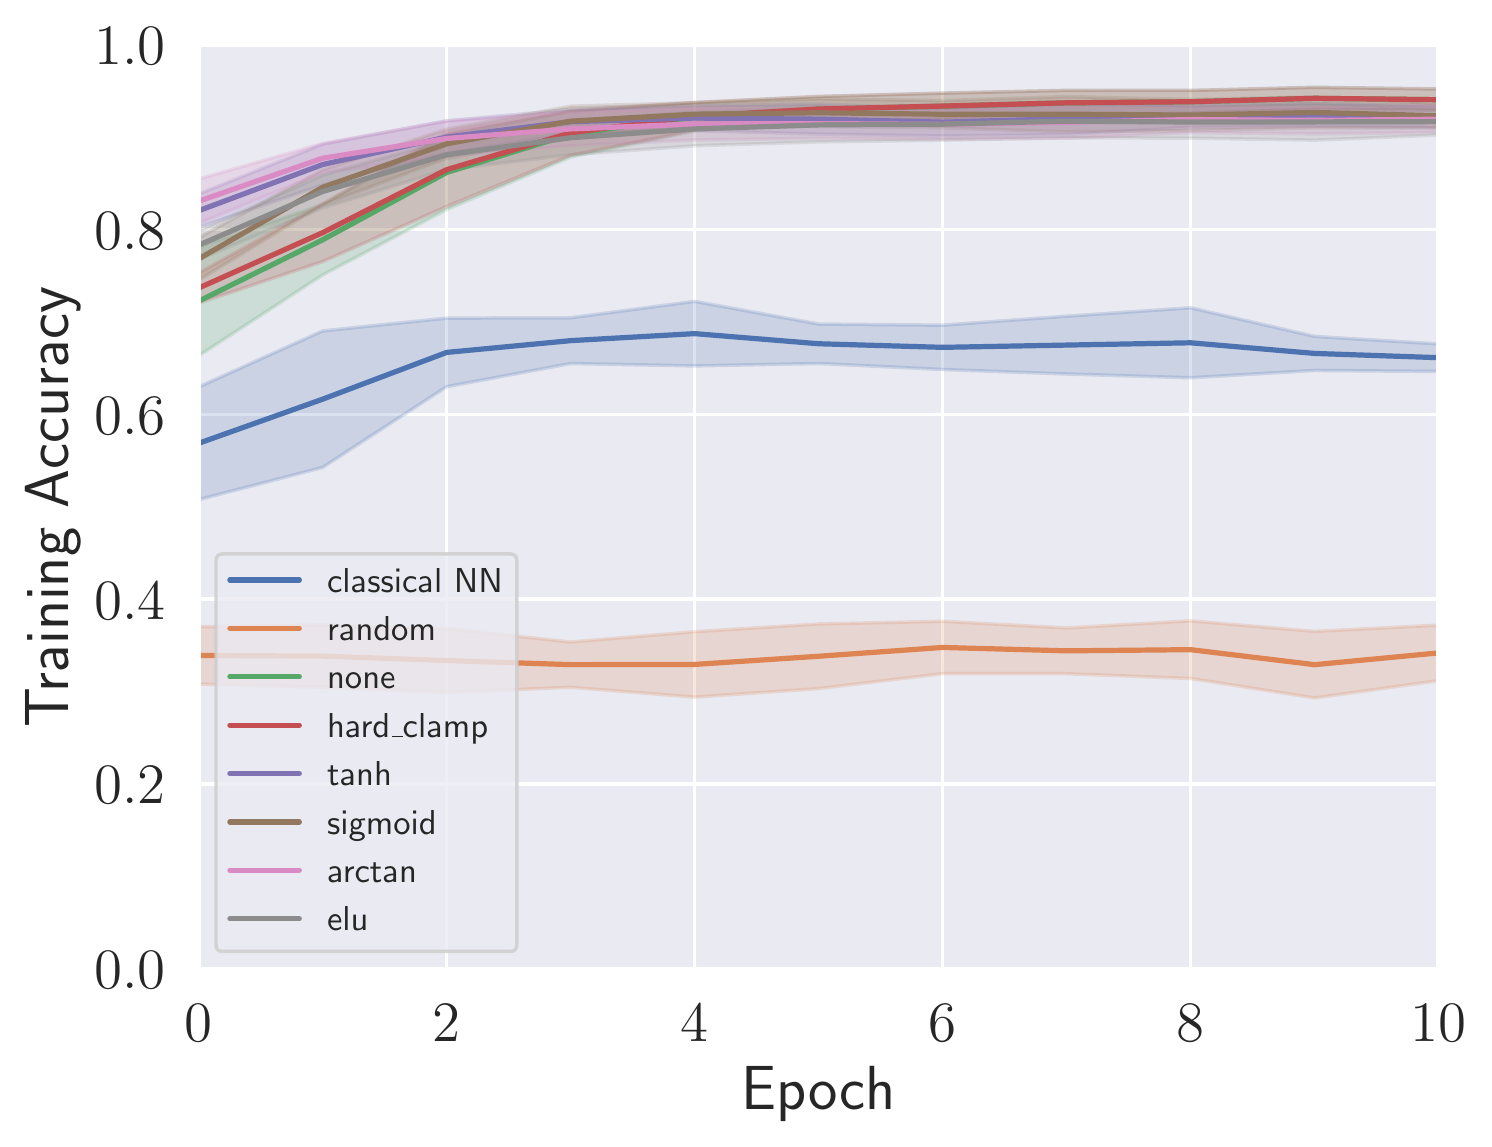}
         \caption{iris valid acc}
         \label{fig:func-id}
     \end{subfigure}
     \begin{subfigure}[t]{0.32\textwidth}
         \centering
         \includegraphics[width=\textwidth]{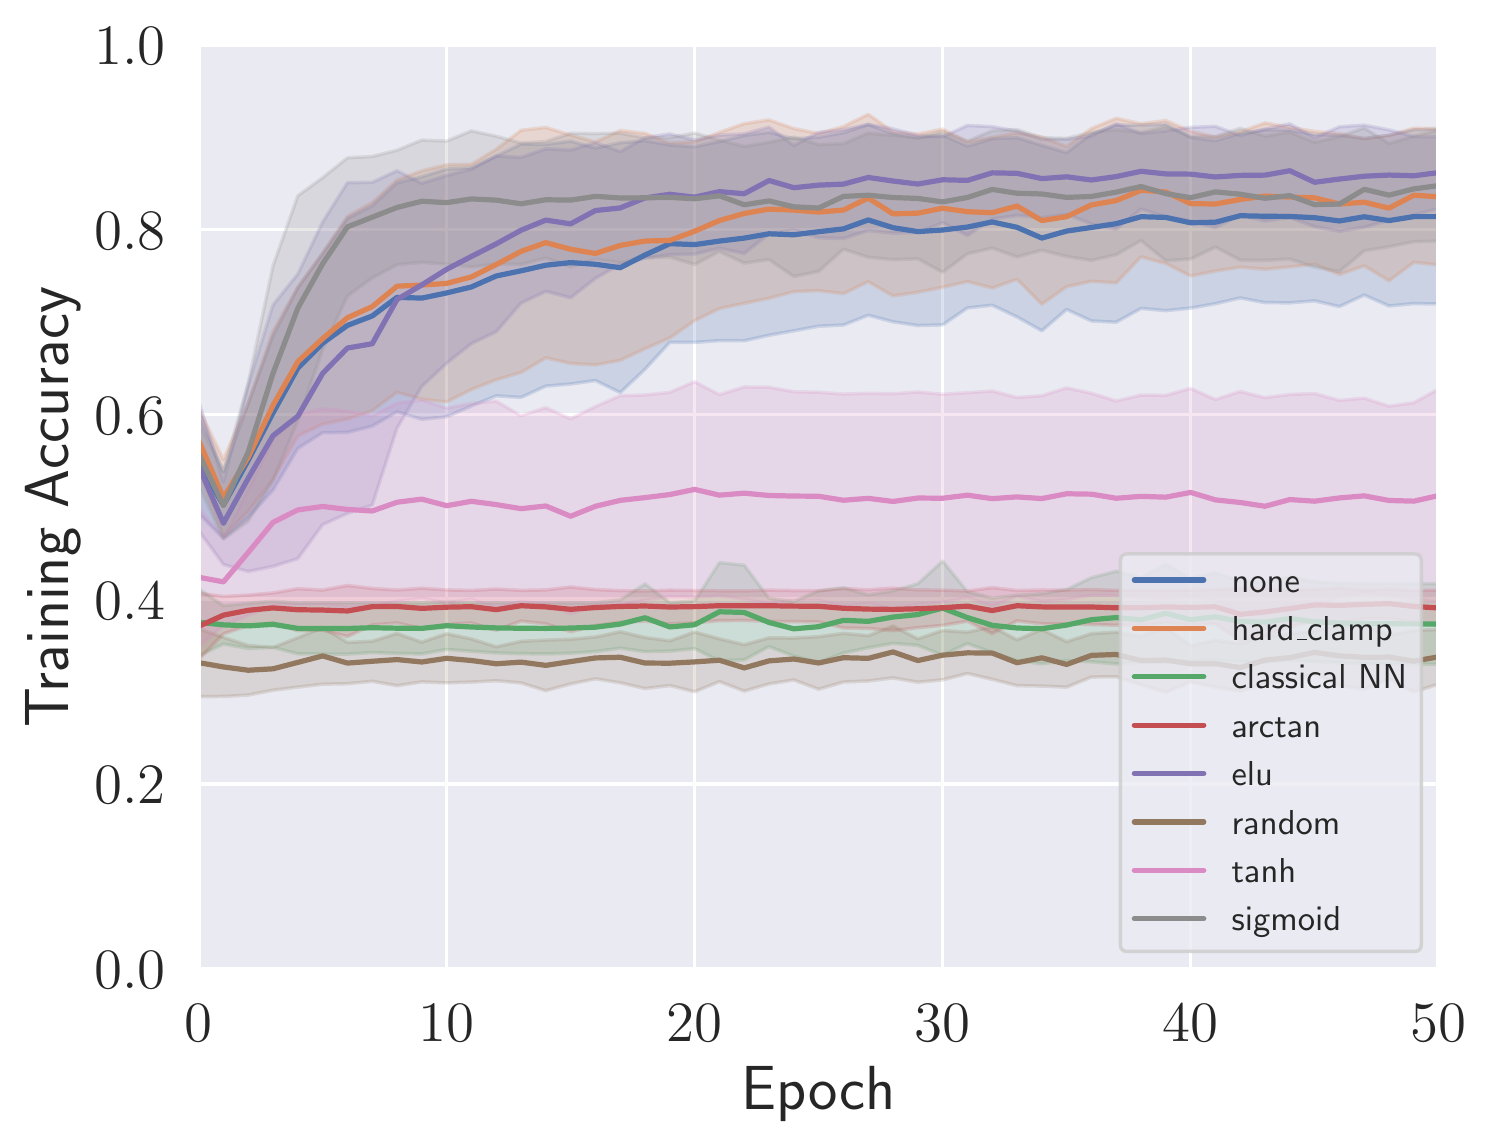}
         \caption{wine valid acc}
         \label{fig:func-clamp}
     \end{subfigure}
     \begin{subfigure}[t]{0.32\textwidth}
         \centering
         \includegraphics[width=\textwidth]{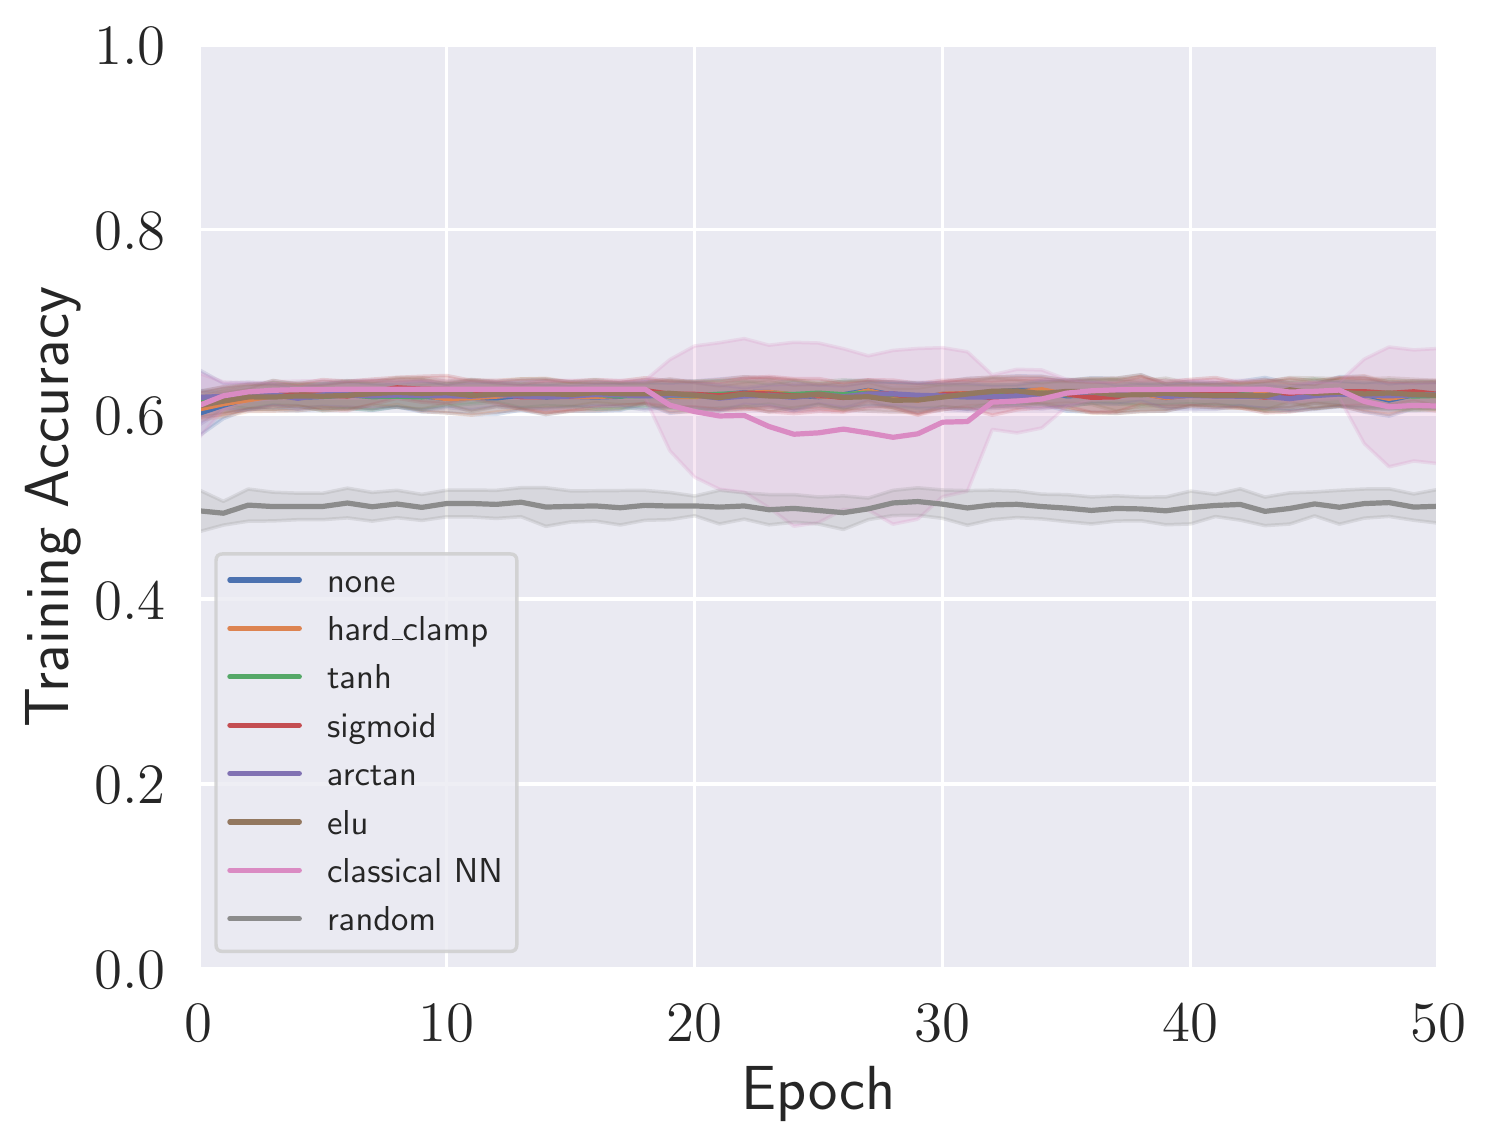}
         \caption{breast cancer valid acc}
         \label{fig:func-tanh}
     \end{subfigure}
     \\
     \begin{subfigure}[t]{0.32\textwidth}
         \centering
         \includegraphics[width=\textwidth]{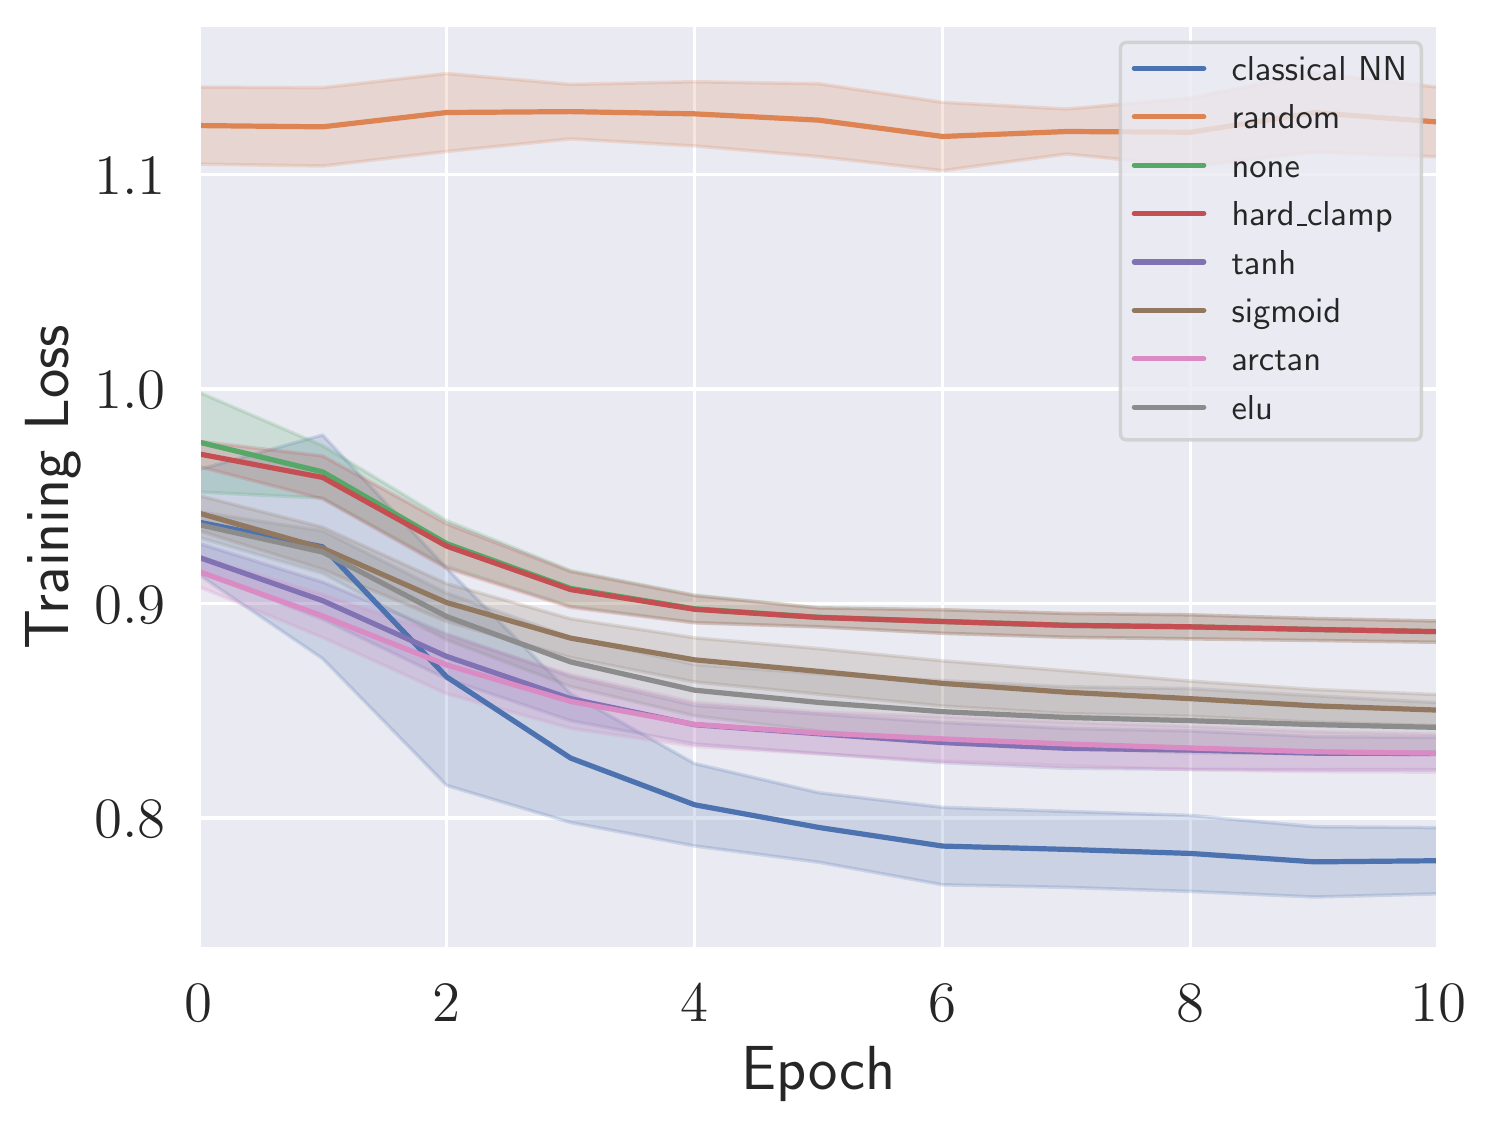}
         \caption{iris valid loss}
         \label{fig:func-arctan}
     \end{subfigure}
     \begin{subfigure}[t]{0.32\textwidth}
         \centering
         \includegraphics[width=\textwidth]{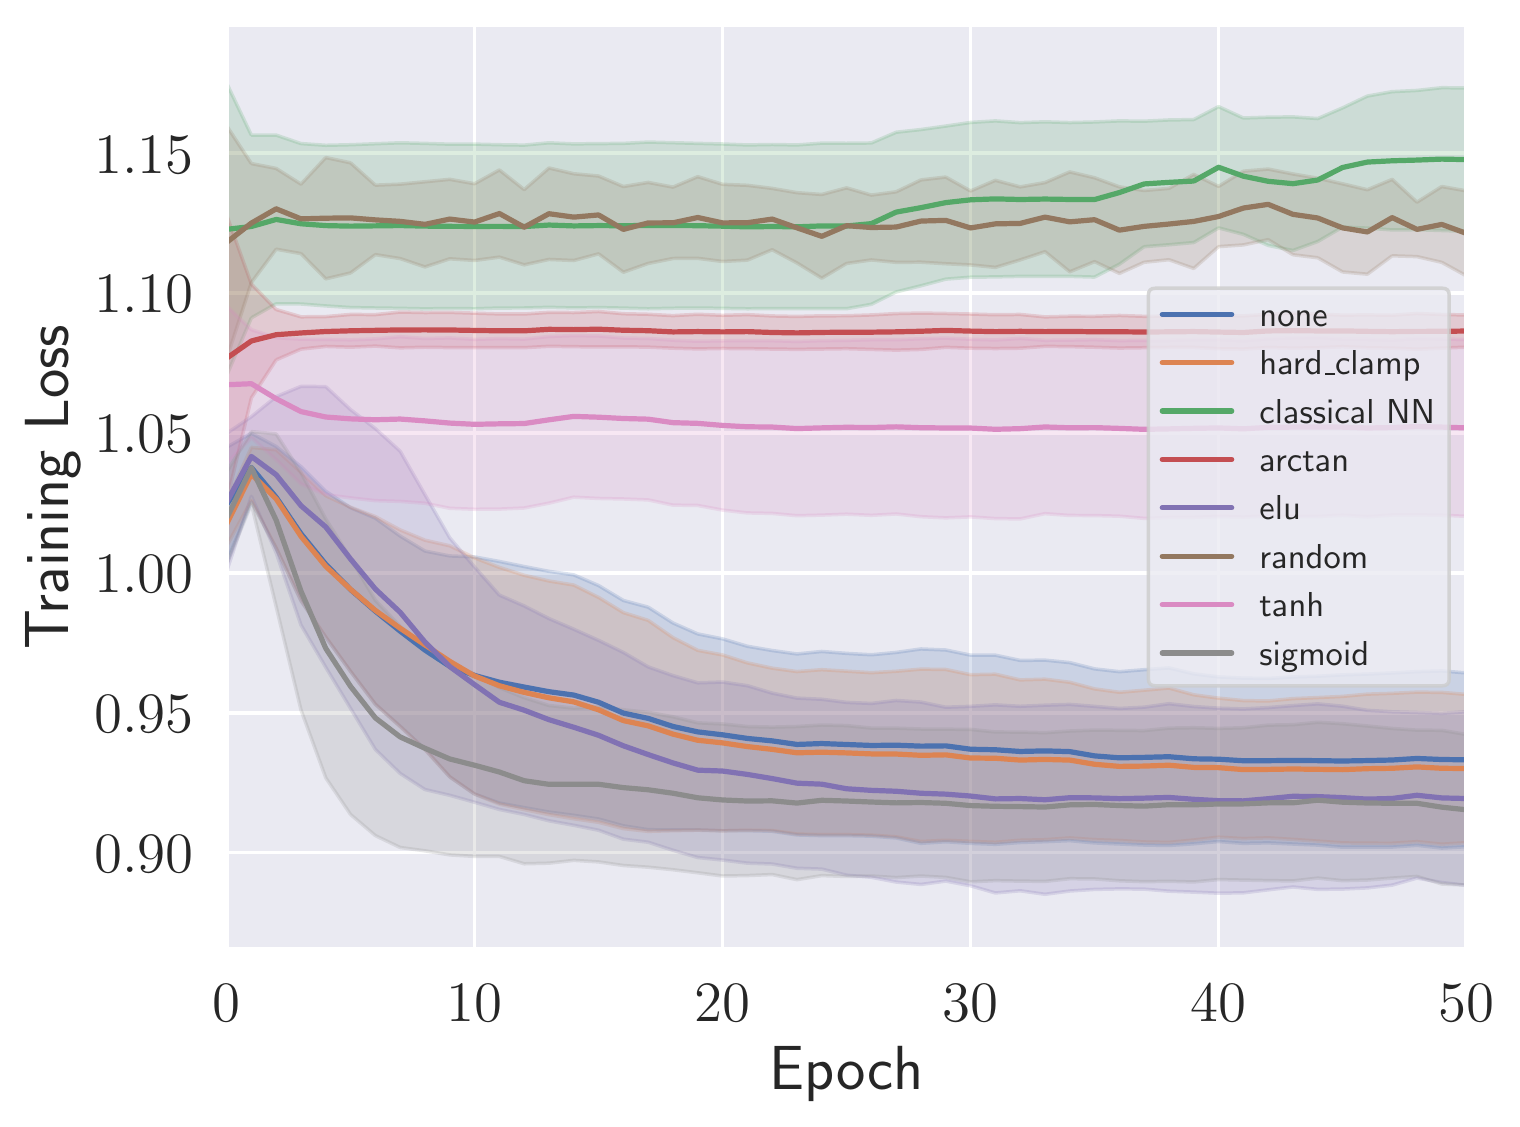}
         \caption{wine valid loss}
         \label{fig:func-sigmoid}
     \end{subfigure}
     \begin{subfigure}[t]{0.32\textwidth}
         \centering
         \includegraphics[width=\textwidth]{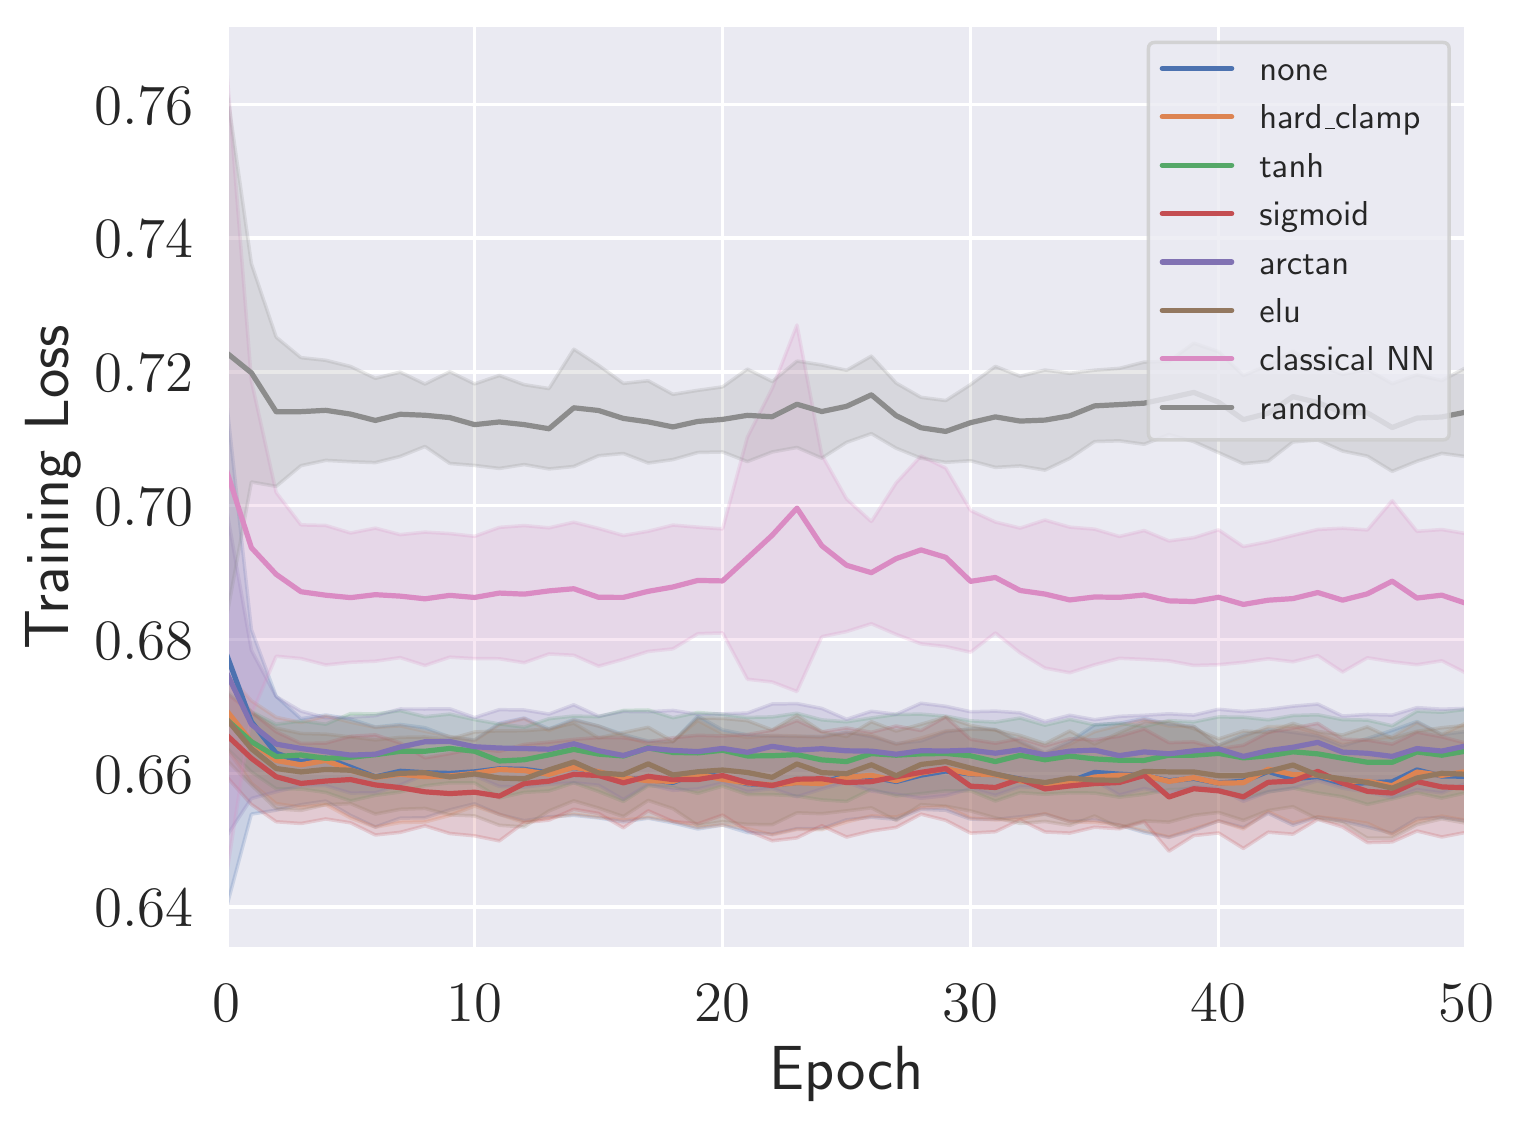}
         \caption{breast cancer valid loss}
         \label{fig:func-elu}
     \end{subfigure}
        \caption{Results for each dataset w/o data re-uploading}
        \label{fig:iris_cf}
\end{figure*}

\begin{figure*}
     \centering
     \begin{subfigure}[t]{0.32\textwidth}
         \centering
         \includegraphics[width=\textwidth]{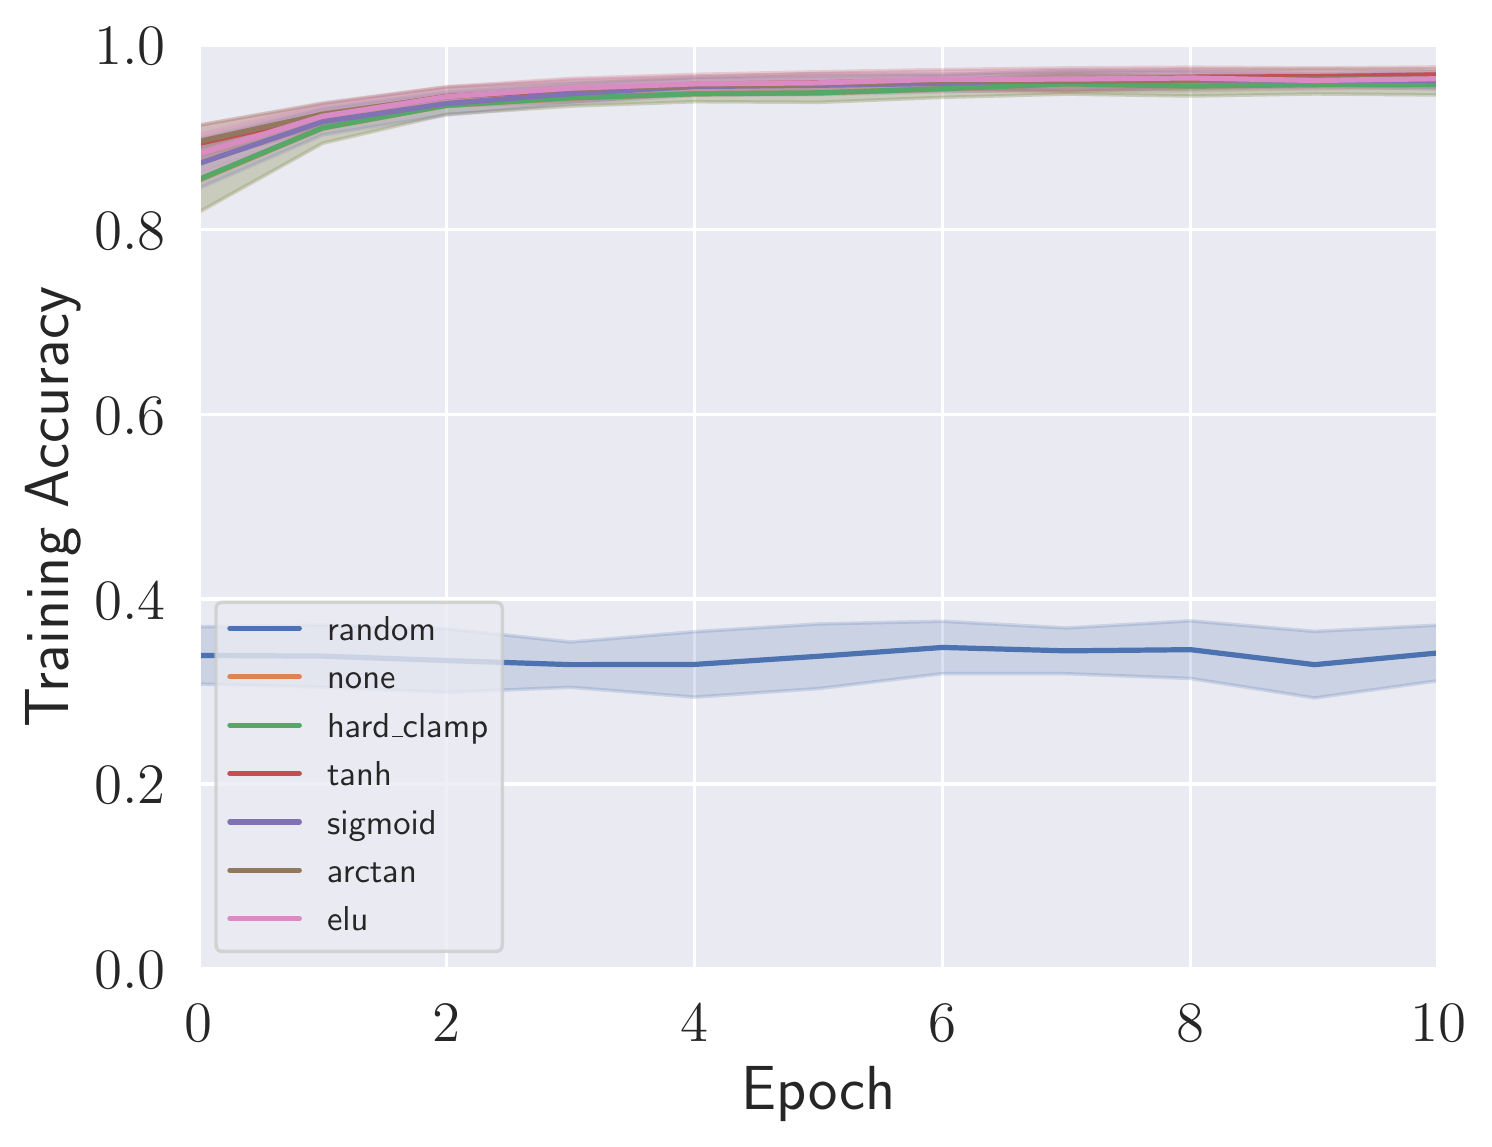}
         \caption{iris valid acc}
         \label{fig:func-id}
     \end{subfigure}
     \begin{subfigure}[t]{0.32\textwidth}
         \centering
         \includegraphics[width=\textwidth]{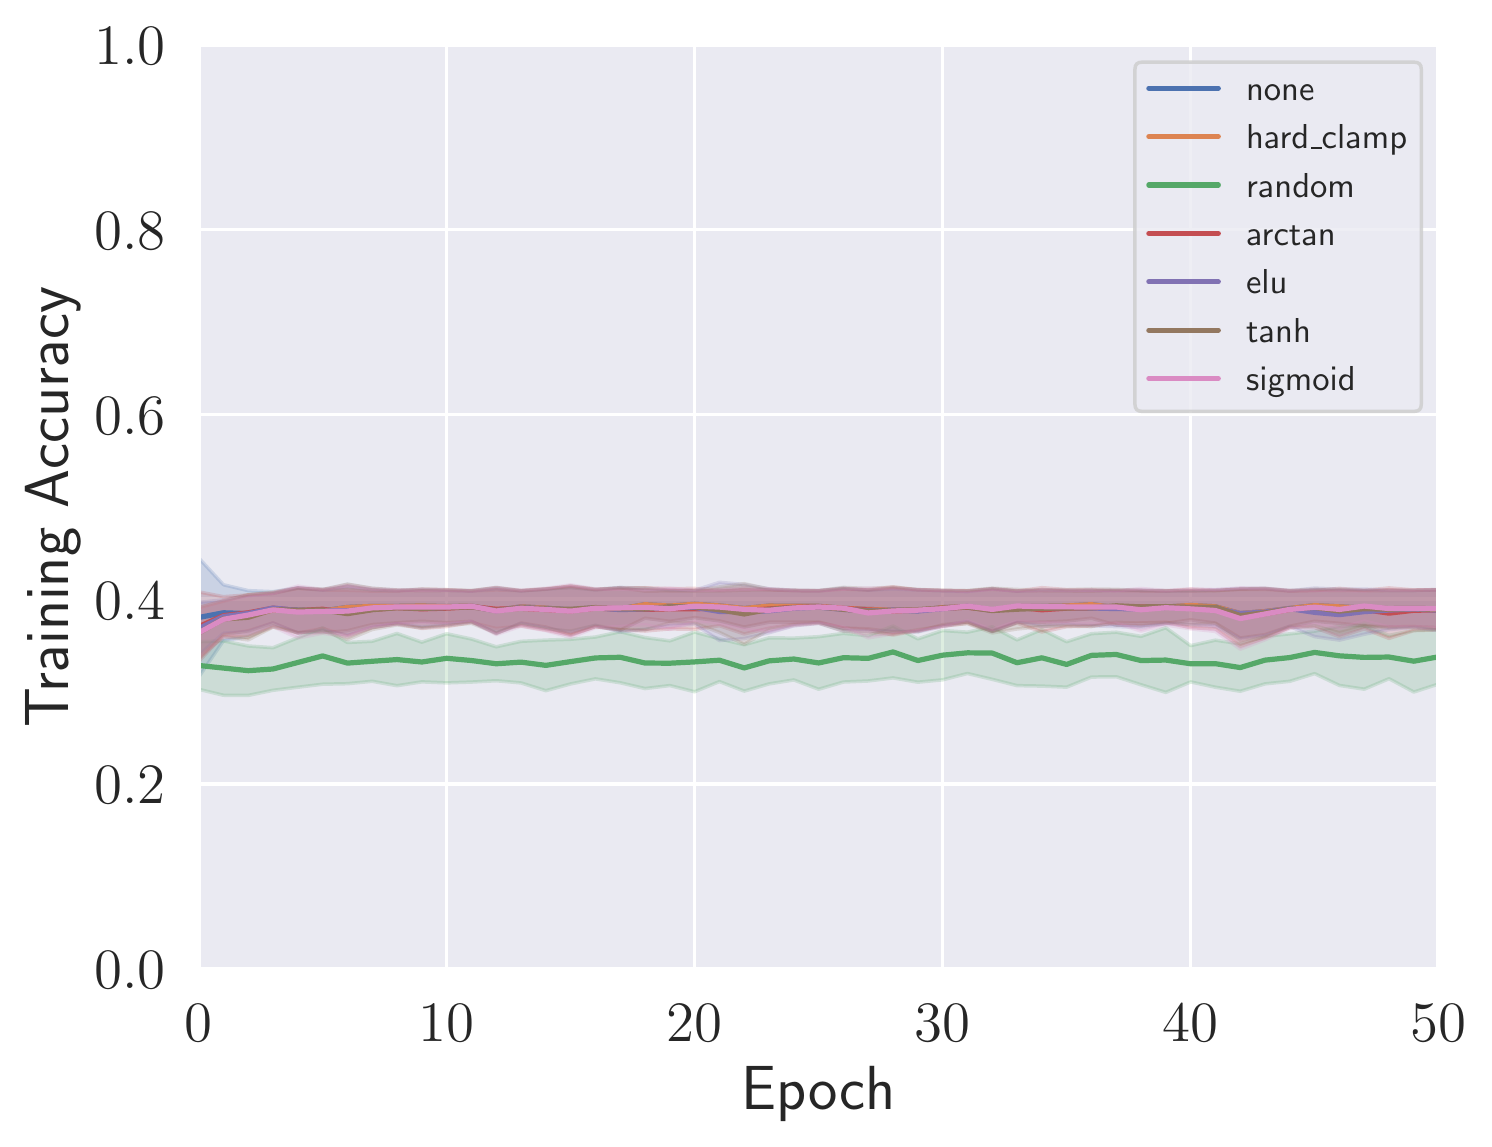}
         \caption{wine valid acc}
         \label{fig:func-clamp}
     \end{subfigure}
     \\
     \begin{subfigure}[t]{0.32\textwidth}
         \centering
         \includegraphics[width=\textwidth]{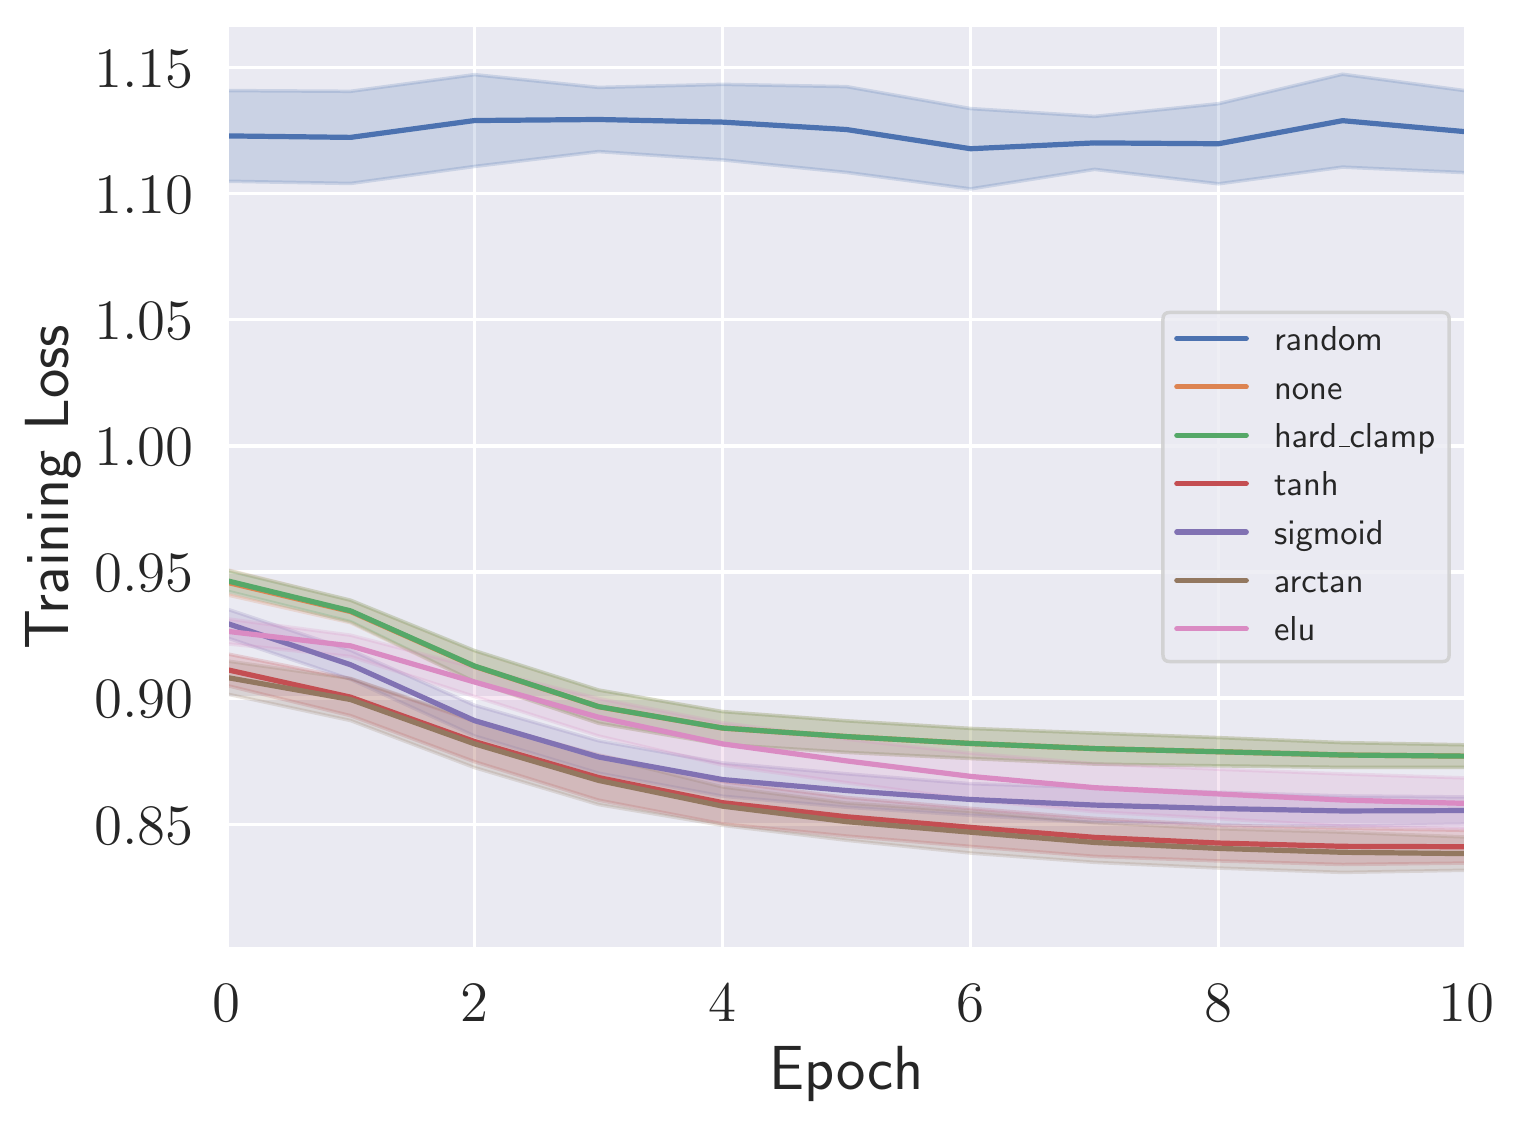}
         \caption{iris valid loss}
         \label{fig:func-arctan}
     \end{subfigure}
     \begin{subfigure}[t]{0.32\textwidth}
         \centering
         \includegraphics[width=\textwidth]{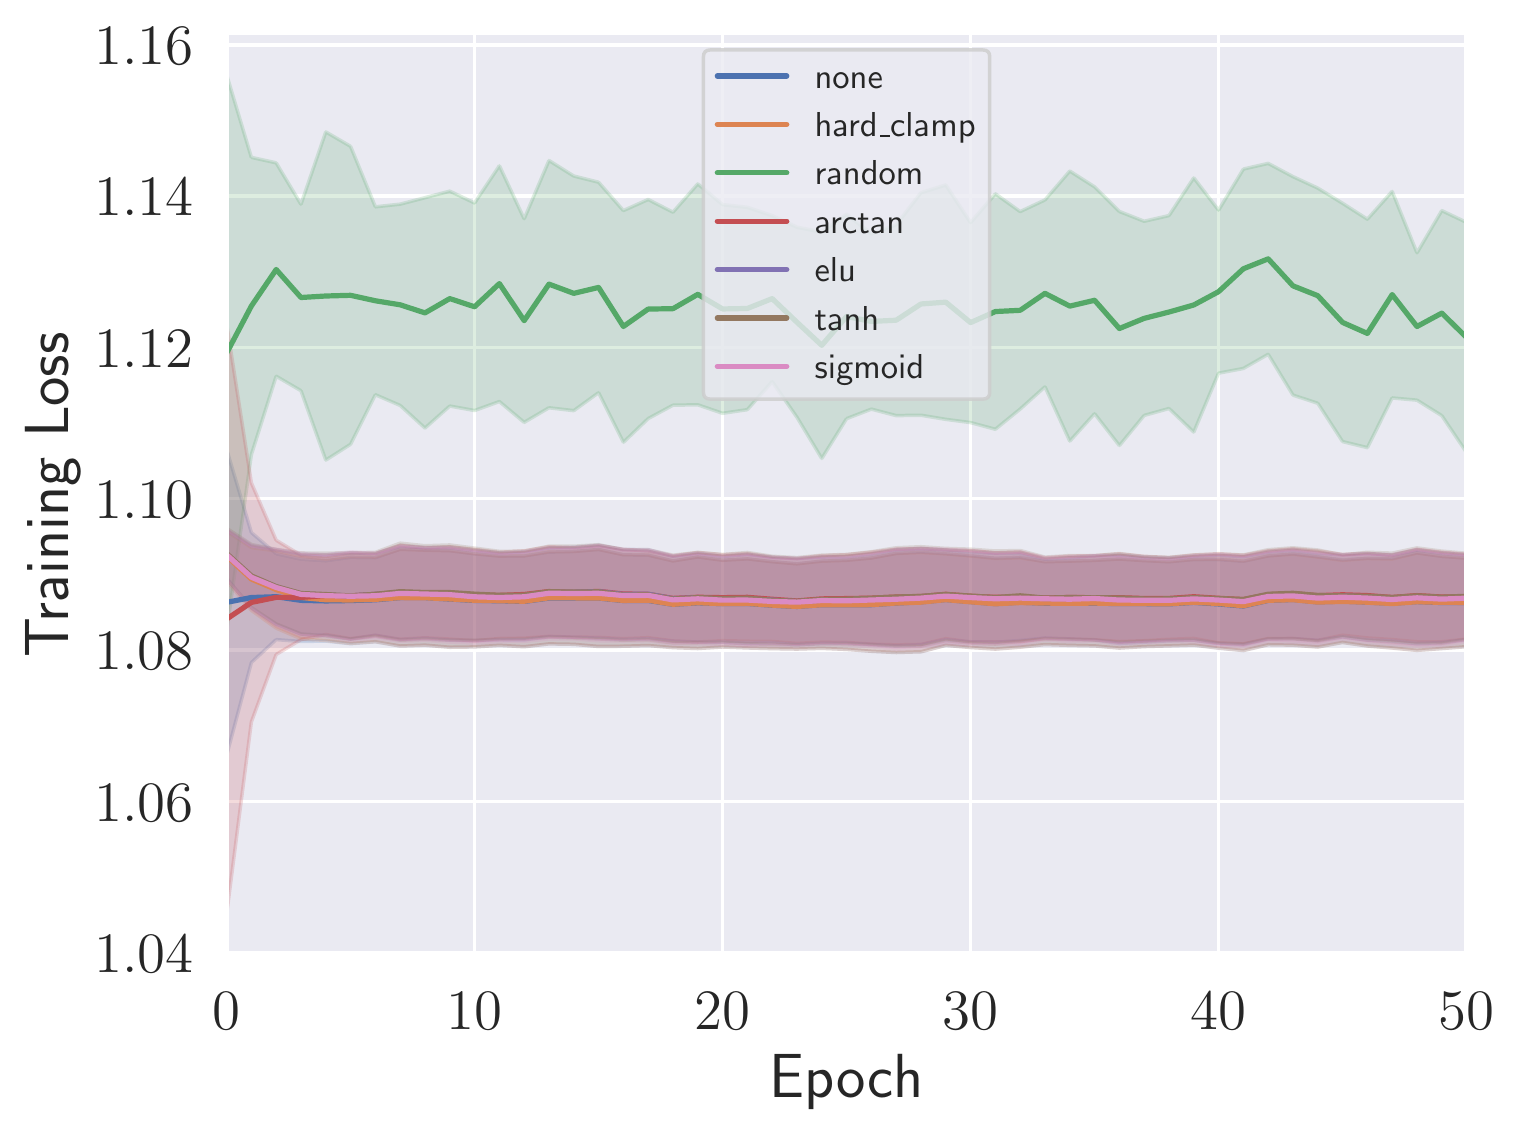}
         \caption{wine valid loss}
         \label{fig:func-sigmoid}
     \end{subfigure}
        \caption{Results for each dataset w/ data re-uploading}
        \label{fig:iris_cf}
\end{figure*}
%%
%\begin{quantikz}
%        \lstick{$q_0$} & \gate{R_x(x_1)} & \gate{R_z(\theta_1^{1})} & \gate{R_y(x_1)}& %\gate{R_z(x_1)}& \ctrl{1}& \qw      & \qw      & \targ{}  &\\
%        \lstick{$q_1$} & \gate{R_x(x_2)} & \gate{R_z(\theta_2^{1})} & \gate{R_y(x_1)}& %\gate{R_z(x_1)}& \targ{} & \ctrl{1} & \qw      & \qw      &\\
%%        \lstick{$q_2$} & \gate{R_x(x_3)} & \gate{R_z(\theta_3^{1})} & \gate{R_y(x_1)}& \gate{R_z(x_1)}& \qw     & \targ{}  & \ctrl{1} & \qw      &\\
%       & & &\ldots& & & &\\
%        \lstick{$q_3$} & \gate{R_x(x_4)} & \gate{R_z(\theta_4^{1})} & \gate{R_y(x_1)}& \gate{R_z(x_1)}& \qw     & \qw      & \targ{}  & \ctrl{-3} &
%    \end{quantikz}
